# Supplementary material for: Quantum State Preparation Using an Exact CNOT Synthesis Formulation
Source: arXiv:2401.01009 source file (2024-01-02)
Supplement: Supplementary file 1 [file appendix-complexity.tex]

\section{Complexity of Amplitude-Preserving Transitions}
In this section, we will discuss the relationship between STAP transitions and general $\text{MCR}_y$ operators. Then, we will demonstrate the efficiency of STAP transitions in terms of transition graph size and the degree of vertices. Finally, we analyze the potential loss in optimality when using STAP transitions.

\subsection{STAP Transitions}
\begin{definition}
    We define \emph{amplitude-preserving}~(AP) mapping between quantum states as a transition where amplitude values are conserved, but the associated basis vectors, or indices, are changed. State transitions between $\psi$ and $\varphi$ is AP if we can express them as $\psi=\sum_xc_x\ket{x}$ and $\varphi=\sum_xc_x\ket{f(x)}$, where $\ket{x}$ and $\ket{f(x)}$ are basis vectors and $c_x$ is the amplitude. A mapping is \emph{single-target amplitude-preserving}~(STAP) if the AP mapping can be implemented using a single-target operator. 
\end{definition}

Notice that a special case of AP transition is when multiple indices map to the same index, i.e., $f(x_1) = f(x_2)$. In this scenario, we should merge their probability instead of an arithmetic summation of their amplitudes to maintain the quantum state's integrity.

\begin{example}
    The state transition from $\ket{\psi} = \sqrt{0.1}\ket{000} + \sqrt{0.1}\ket{001} + \sqrt{0.3}\ket{010} + \sqrt{0.5}\ket{110}$ to state $\ket{\varphi} = \sqrt{0.2}\ket{000} + \sqrt{0.3}\ket{010} + \sqrt{0.5}\ket{110}$ can be implemented using a STAP operator because we can find an index mapping $f = \{\ket{000}\rightarrow\ket{000}, \ket{001}\rightarrow\ket{000}, \ket{010}\rightarrow\ket{010}, \ket{110}\rightarrow\ket{110}\}$ that transform $\psi$ to $\varphi$ without changing the magnitudes of their amplitudes. To merge the amplitudes $c_{000} = \sqrt{0.1}$ and $c_{001}= \sqrt{0.1}$, the operation rotates the last qubit by $\theta\!=\!-2\cdot \arctan{\sqrt{\frac{0.1}{0.1}}}\!=\!-\frac{\pi}{2}$. Therefore, this STAP operator can be implemented using a Y rotation gate, $R_y(-\frac{\pi}{2})$, targeting the last qubit and controlled by the second qubit. 
    \begin{equation*}
        \small
        \Qcircuit @C=.7em @R=1em {
        \lstick{q_1:} & \qw &  \qw      & \qw \\ 
        \lstick{q_2:} & \qw & \ctrlo{1} & \qw \\
        \lstick{q_3:} & \qw & \rypi{2}  & \qw
        } \qquad \hspace{3em}
        \Qcircuit @C=.7em @R=1em {
         \lstick{q_1:} & \qw & \qw      & \qw       & \qw       & \qw       & \qw \\ 
         \lstick{q_2:} & \qw & \qw      & \ctrlo{1} & \qw       & \ctrlo{1} & \qw \\
         \lstick{q_3:} & \qw & \rypi{4} & \targ     & \rypi{4}  & \targ     & \qw
        }
    \end{equation*}
    Above are the circuit and the corresponding decomposition into $\{\text{CNOT}, \mathcal{U}(2)\}$. Since the MCR$_y$ has one control qubit, the CNOT cost is $2$. 
\end{example}

% \begin{definition}
%     Let $c_1$ and $c_2$ be the amplitudes of two indices, $x_1$ and $x_2$, that map to the same index, i.e., $f(x_1) = f(x_2)$.
% \end{definition}

\begin{observation}\label{obs:stap-mcry-cases}
    Let $q_i$ be the target qubit of the STAP transition. As shown in Lemma~\ref{lemma:mcry-gate-are-sufficient}, we can represent the STAP using a rotation table for $q_i$. Let $\alpha\ket{0}+\beta\ket{1}$ be the initial state of $q_i$ corresponds to an index $\ket{x}$. All possible outcomes of an amplitudes-preserving transition and their corresponding rotation angle are:
    \begin{enumerate}
        \item $\alpha\ket{0}+\beta\ket{1}$: $\theta_x=0$.
        \item $\alpha\ket{0}+\beta\ket{0}$: $\theta_x=-2\arctan\frac{\beta}{\alpha}$.
        \item $\alpha\ket{1}+\beta\ket{1}$: $\theta_x=\pi-2\arctan\frac{\beta}{\alpha}$.
        \item $\alpha\ket{1}+\beta\ket{0}$: Pauli-X.
    \end{enumerate}
    For the special case where initial state of $q_i$ is $\ket{0}$ or $\ket{1}$, the outcome of an AP transition is also $\ket{0}$ or $\ket{1}$, which correspond to case 1) and 4). Therefore, AP transitions only ``merge'' the indices and cannot ``split'' the indices. As a result, if a state transitions from $\psi$ to $\varphi$ is AP, then $S(\varphi)\subseteq S(\psi)$ and $|S(\varphi)|\leq |S(\psi)|$.
\end{observation}

\begin{lemma}\label{lemma:graph-size-of-stap}
    The number of reachable states from a state $\psi$ using gates in $\{\text{STAP}\}$ is bounded by $2^{nm}$, where $n$ is the number of qubits and $m$ is the cardinality of $\psi$'s index set, i.e., $m=|S(\psi)|$.
\end{lemma}
\begin{proof}
    Observe that there are $2^{mn}$ different possible mappings as the cardinality of the domain is $m$, and the cardinality of the target is $2^n$. Therefore, it suffices to show both statements below hold:
    \begin{enumerate}
        \item The transition using a sequence of STAP transitions remains to be AP. 
        \item Each mapping represents at most one quantum state.  
    \end{enumerate}
    Statement 1) holds because applying two AP transitions with index mapping function $f$ and $g$ consecutively is equivalent to an AP transition with mapping $g\circ f$, which maps $\sum_xc_x\ket{x}$ to $\sum_xc_x\ket{g(f(x))}$.

    Statement 2) holds by definition if all indices after mapping are different. To complete the proof, we discuss the case where multiple indices map to the same index, i.e., $f(x_1) = f(x_2)$ with amplitudes $c_1$ and $c_2$. The amplitudes after merging them have two possible values, $+\sqrt{c_1^2+c_2^2}$ or $-\sqrt{c_1^2+c_2^2}$. \todo{(low-prio) how to show that this minus sign does not matter (without introducing Pauli-Z gates?)} \note{in the worst case, we can weaken the lemma and show that the number of the reachable states is bounded by $2^{m\cdot(n+1)}$ because of the plus-minus sign.}    
\end{proof}

\begin{lemma}\label{lemma:degree-of-stap}
    The maximal degree of vertices in the state transition graph of $\{\text{STAP}\}$, which is the maximal number of adjacent states, is bounded by $2^m\cdot n$, where $n$ is the number of qubits and $m$ represents the cardinality of the state's index set. \note{do I need to repeat these definitions in every lemma?}
\end{lemma}
\begin{proof}
    During a STAP transition targeting qubit $q_i$, each of the $m$ indices can decide whether to flip the $i$th bit. Therefore, $2^m$ different combinations of STAP transitions result in $2^m$ different states. Combining all $n$ possible qubits as the target, the maximal degree of a vertex is bounded by $2^m\cdot n$.
\end{proof}
