# Supplementary material for: Quantum State Preparation Using an Exact CNOT Synthesis Formulation
Source: arXiv:2401.01009 source file (2024-01-02)
Supplement: Supplementary file 2 [file appendix-mcry.tex]

\section{Optimal MCR$_y$ Decomposition for QSP}\label{sec:optimal-mcry-decomposition}
In this section, we first introduce the existing method to find the optimal CNOT number to decompose a \emph{single-target multi-controlled Y rotation gate}~(MCR$_y$) using $\mathcal{L} = \{\text{CNOT}, \text{R}_y\}$. Then, we propose a decomposition algorithm specialized to the \emph{real quantum state preparation problem}~(real QSP). Leveraging the don't care in real QSP, our algorithm finds the circuit with the minimum number of CNOT gates for the decomposition. Moreover, we discuss the relationship between MCR$_y$ decomposition and the exact CNOT synthesis method introduced in \Cref{sec:algorithm}.

\begin{definition}
    A general MCR$_y$ operator can be represented by a mapping between the control index and corresponding rotation angles, i.e., $f:S\rightarrow [0,2\pi)$. We use \emph{rotation table} as a canonical representation of the mapping. When the control qubits are in state $\ket{x}$, the corresponding rotation angle is $\theta = f(\ket{x})$ and a $\text{R}_y(\theta)$ is applied to the target qubit.
\end{definition}

The key difference between our general MCR$_y$ operator and the C$^n$R$_y$ operator in the literature is that C$^n$R$_y$ applies one rotation angle to a specific control qubit state while MCR$_y$ can apply at most $2^n$ different rotations for different conditions, where $n$ is the number of control qubits. 

The qubit reduction method utilizes MCR$_y$ to entangle or disentangle qubits in QSP~\cite{mozafari2019preparation}. For example, to prepare the state $\psi = \alpha\ket{00}\otimes\ket{0}_3 + \beta\ket{01}\otimes\ket{+}_3 + \gamma\ket{10}\otimes\ket{-}_3$,
from the state $\varphi = (\alpha\ket{00}+\beta\ket{01}+\gamma\ket{10})\otimes\ket{0}_3$ by entangling $q_3$ to the system, we can express the transition as a rotation table with respect to $q_3$.

\begin{table}[h]
\normalsize
    \centering
    \begin{tabular}{l|cccc}
    \hline
        Control index $q_1,q_2$         & $\ket{00}$       & $\ket{01}$  &$\ket{10}$  &$\ket{11}$  \\
        Rotation angle & $0$ &    $\frac{\pi}{2}$      & $\frac{3\pi}{2}$    &   X  \\
    \hline
    \end{tabular}
    \caption{An example of a rotation table.}\label{tab:rotation-table}
\end{table}
``X'' represents don't care. The rotation angle when the control qubits are $\ket{11}$ does not matter because the probability of observing $\ket{11}$ is $0$. 

\subsection{Gray Code Decomposition}
The previous method first assumes a fixed template based on the bit flipping in Gray code for decomposition. 
\begin{figure}[h]
\centering
\mbox{
\small
    \Qcircuit @C=.7em @R=1em {
         \lstick{q_1:} & \qw & \qw           & \qw          & \qw           & \ctrl{2}  & \qw           & \qw       & \qw           & \ctrl{2}   & \qw \\ 
         \lstick{q_2:} & \qw & \qw           & \ctrl{1}     & \qw           & \qw       & \qw           & \ctrl{1}  & \qw           & \qw        & \qw \\
         \lstick{q_3:} & \qw & \ry{\theta_1} & \targ        & \ry{\theta_2} & \targ     & \ry{\theta_3}  & \targ    & \ry{\theta_4} & \targ      & \qw
    }
}
\caption{\small MCR$_y$ decomposition using the Gray code template.}\label{fig:gray-code}
\end{figure}
Then, we have the following constraints for the angles and find a feasible assignment for the rotation angles:
\begin{equation*}
\left\{
\begin{array}{rl}
    \theta_1 + \theta_2 + \theta_3 + \theta_4 &= 0 \\
    \theta_1 - \theta_2 - \theta_3 + \theta_4 &= \frac{\pi}{2} \\
    \theta_1 + \theta_2 - \theta_3 - \theta_4 &= \frac{3\pi}{2}
\end{array}
\right. \Rightarrow
\left\{
\begin{array}{rl}
    \theta_1 &= \frac{\pi}{4} \\
    \theta_2 &= \frac{\pi}{2} \\
    \theta_3 &= -\frac{3\pi}{4} \\
    \theta_4 &= 0
\end{array}
\right.
\end{equation*}

This method requires $2^n$ CNOTs to decompose the MCR$_y$ gates, where $n$ is the number of control qubits, regardless of the values of rotation angles and don't cares. 

\subsection{Leveraging Don't Cares in MCR$_y$ Decomposition}
Note that QSP problems assume all circuits are initialized to the ground state $\ket{0}$. Therefore, let $U$ be the unitary matrix of the entire circuit; only the first row of $U$ affects the final state. For example:
\begin{equation*}
    H=\frac{1}{\sqrt{2}}\begin{pmatrix}
        1 & 1 \\
        1 & -1 
    \end{pmatrix}\quad\text{and}\quad
    \text{R}_y(\frac{\pi}{2}) = \begin{pmatrix}
        \cos\frac{\pi}{4} & \sin\frac{\pi}{4} \\
        -\sin\frac{\pi}{4} & \cos\frac{\pi}{4} 
    \end{pmatrix}
\end{equation*}
has the same effect on $\ket{0}$. 

The portion of the care set decays exponentially as the number of qubits increases. As a result, leveraging don't cares in QSP can significantly improve the circuit's quality. For example, the circuit in \Cref{fig:exact-synthesis-mcry} can replace \Cref{fig:gray-code} if the initial state of $q_3$ is $\ket{0}$ and reduce the number of CNOT gates from $4$ to $2$.
\begin{figure}[t]
\centering
\mbox{
\small
    \Qcircuit @C=.7em @R=1em {
         \lstick{q_1:} & \qw & \qw           & \ctrl{2}          & \qw           & \qw  & \qw           &  \qw \\ 
         \lstick{q_2:} & \qw & \qw           & \qw     & \qw       & \ctrl{1}     & \qw                 &  \qw \\
         \lstick{q_3:} & \qw & \ry{-\frac{\pi}{4}} & \targ        & \ry{\frac{\pi}{2}} & \targ     & \ry{-\frac{\pi}{4}} &  \qw
    }
}
\caption{MCR$_y$ decomposition using exact synthesis.}\label{fig:exact-synthesis-mcry}
\end{figure}

\begin{observation}\label{obs:unitary-is-ry}
    As introduced in \Cref{sec:background}, $\text{R}_y$ gates are sufficient to implement all single-qubit gates in $\mathcal{U}(2)$ if the initial state is fixed. 
\end{observation}

\begin{lemma}\label{lemma:mcry-gate-are-sufficient}
    MCR$_y$ gates are sufficient to represent all single-target state transitions in real QSP, i.e., real state preparation with all operations in the X-Y plane.
\end{lemma}
\begin{proof}
    A single-target transition can be expressed as:
    \begin{equation*}
        \ket{\psi} = \sum_{x\in S}(\ket{x}\otimes\ket{\psi_x}) \rightarrow \sum_{x\in S}(\ket{x}\otimes\ket{\varphi}) = \ket{\varphi},
    \end{equation*}
    where $S$ represents the care set of control qubit indices. In real QSP, $\psi_x$ and $\varphi_x$ are known single-qubit states of the target qubit. 

    According to Observation~\ref{obs:unitary-is-ry}, the unitary $U=\ket{\varphi_x}\bra{\psi_x}+\ket{\varphi_x^\perp}\bra{\psi_x^\perp}$ can be implemented by a $\text{R}_y$ gate with rotation angle $\theta_x$. Therefore, we can find a rotation table that indicates the angle $\theta_x$ for each $\ket{x}$, which is implemented by a MCR$_y$ gate. 
\end{proof}

\subsection{An Exact Synthesis Algorithm for MCR$_y$ Decomposition}\label{subsec:exact-synthesis-algorithm}
As shown in \Cref{alg:exact-mcry-decomposition}, given a target rotation table, our exact synthesis algorithm:
\begin{enumerate}
    \item defines a hyper-parameter $K$ as the number of CNOTs in the template and initializes it to $K=0$. 
    \item constructs an equality system to check if the rotation table can be implemented if using $K$ CNOTs.
    \item analyzes the result. If a set of solutions is found, we return the circuit with $K$ CNOTs. Otherwise, we increase $K$ by one and repeat step 2).
\end{enumerate}

\begin{algorithm}[t]
\caption{Exact MCR$_y$ decomposition}\label{alg:exact-mcry-decomposition}
\SetKwInOut{Input}{input}
\SetKwInOut{Output}{output}

 \DontPrintSemicolon
 \Input{The rotation table $f$ with $n$ control qubits.}
 \Output{A sequence of quantum operators to prepare the rotation table with $K$ CNOTs.}
 
$K \gets 0$ \;
$\text{solution} \gets \varnothing$ \;
\While{$\text{solution}$ is $\varnothing$} {
    \For{$\{S_k\}$ in {$\mathbb{Z}_{n}^{\otimes K}$}} {
        $M \gets $ Construct equality system ($f$, ${S_k^i}$)\;
        solution $\gets $ Solve($M$) \;
    }
    $K \gets K+1$ \;
}
\Return solution.\;
\end{algorithm}

All utilized variables are listed in \Cref{tab:variable-declaration-mcry-decomposition}. In the rest of this section, we will detail these definitions. 
\begin{table}[b]
\small
    \centering
    \begin{tabular}{lll}
    \hline
    $S^i_k$ & $\{0,1\}$ & Whether $q_i$ is the control qubit in the $k$th CNOT.\\
    $R^x_k$ & $\{-1,1\}$ & Whether $\ket{x}$ is enabled in the $k$th CNOT. \\
    $\varphi^x_k$ & $[0, 2\pi)$ & The angle corresponds to $\ket{x}$ after the $k$th CNOT. \\
    $\theta_k$ & $[0, 2\pi)$ & The rotation angle of R$_y$ after the $k$th CNOT. \\
    \hline
    \end{tabular}
    \caption{\small Variable declaration for the exact MCR$_y$ decomposition.}
    \label{tab:variable-declaration-mcry-decomposition}
\end{table}

\noindent\textbf{\textit{C1-}CNOT variables and constraints}. 

We assume that all the CNOT gates in the circuit target the same qubit. 
\todo{can we prove that the target qubit of all CNOTs is the same in the optimal solution to decompose single-target MCRy, or it is just an assumption?}
Therefore, the control qubit suffices to represent a CNOT gate. We define CNOT variables, $S^i_k$, as a binary value that indicates whether $q_i$ is the control qubit in the $k$th CNOT. Since a CNOT has only one control qubit, we have:
\begin{equation*}
    \sum_{i\in \mathbb{Z}_{n}}S^i_k = 1, \forall k\in \mathbb{Z}_{K},
\end{equation*}
where $n$ is the number of the candidate control qubits. The control qubit determines the set of indices that are affected by the CNOT. More specifically, we let the variable $R^x_k = -1$ if the index $\ket{x}$ is enabled by the $k$th CNOT and $1$ otherwise. We get:
\begin{equation}\label{eqn:r-s-variable-relation}
    R^{x}_{k} := (-1)^{\sum_{i\in \mathbb{Z}_{n}} S^i_k\cdot[x]_i}, 
\end{equation}
where $[x]_i$ represents the value of the $i$th bit of $x$ in the binary form. 

\noindent\textbf{\textit{C2-}Rotation angle variables and constraints}. 

We use $\varphi_x^k$ to represent the rotation angle corresponding to index $\ket{x}$ after the $k$th CNOT gate. The values of the initial and final angles, $\varphi_x^0$ and $\varphi_x^K$, are given. 

Then, we define rotation angle constraints as shown in \Cref{eqn:rotation-angle-constraints}\footnote{We can easily modify the rotation angle constraints to target the library $\{CZ, \text{R}_{y}\}$. $\varphi_x^{k+1} = \theta^k + R_x^k\cdot(\varphi_x^{k}).$ The difference between CNOT(CX) and CZ is the $\frac{\pi}{2}$ offset of the reflection axis.}. 
\begin{equation}\label{eqn:rotation-angle-constraints}
    \varphi^x_{k+1} = \frac{\pi}{2} + \theta_k + R^x_k\cdot(\varphi^x_{k}-\frac{\pi}{2}). 
\end{equation}
This constraint describes the evolution of the rotation table before and after the $k$th CNOT gate. If the index $\ket{x}$ is not enabled by the CNOT, then $R^x_k = 1$, and $\varphi^x_{k+1} = \varphi^x_{k} + \theta_k$ because of the R$_y$ gate after CNOT. Otherwise, if $\ket{x}$ is enabled, $R^x_k = -1$, then $\varphi^x_{k+1} = \pi - \varphi^x_{k} + \theta_k$ because the CNOT gate reflect the previous angle along $\varphi = \frac{\pi}{2}$ before applying the R$_y$ gate. 

% The minimum number of CNOTs to decompose an MCR$_y$ depends on the care set's cardinality and the algebraic relationship between the rotation angles. 

\begin{example}\label{example:exact-mcry-decomposition}
    Given the rotation table from \Cref{tab:rotation-table}, and the initial state of $\ket{0}_3$, we can assign the initial and final values to the rotation angle variables. Assume we are at the iteration where $K=2$, then:
    \begin{equation*}
        \varphi^{00}_0 = \varphi^{01}_0 = \varphi^{10}_0 = \theta_0\,,\, \varphi^{00}_2 = 0,\,\varphi^{01}_2 = \frac{\pi}{2},\,\varphi^{10}_2 = \frac{3\pi}{2}, 
    \end{equation*}
    where $\theta^0$ is the offset introduced by the first R$_y$ gate. Since $\ket{11}$ is a don't care, we can exclude it from the equality system or leave it as a free variable. 

    The target is to find an assignment to $\theta_0$, $\theta_1$, $\theta_2$, $S^i_1$, and $S^i_2$, such that the equality system is satisfied. For clarity, we assume the control qubits of the two CNOTs are $S^1_1\!=\!1$ and $S^2_2\!=\!1$. Therefore, $R^{00}_1\!=\!R^{01}_1\!=\!R^{00}_2\!=\!R^{10}_1\!=\!1$ and $R^{10}_1\!=\!R^{01}_2=-1$. We can simplify the equality system by plugging in the known variables and canceling intermediate variables as shown in \Cref{eqn:equality-system-example}.
    \begin{equation}\label{eqn:equality-system-example}
        \left\{
        \begin{array}{rl}
            \varphi^{00}_{1}&=\varphi^{00}_{0} + \theta_1  \\
            \varphi^{01}_{1}&=\varphi^{01}_{0} + \theta_1  \\
            \varphi^{10}_{1}&=\pi - \varphi^{10}_{0} + \theta_1  \\
            \varphi^{00}_{2}&=\varphi^{00}_{1} + \theta_2  \\
            \varphi^{01}_{2}&=\pi - \varphi^{01}_{1} + \theta_2  \\
            \varphi^{10}_{2}&=\varphi^{10}_{1} + \theta_2  \\
        \end{array}
        \right. \rightarrow
        \left\{
        \begin{array}{rl}
            0&=\theta_0 + \theta_1 + \theta_2  \\
            \frac{\pi}{2}&=\pi - (\theta_0 + \theta_1) + \theta_2  \\
            \frac{3\pi}{2}&=(\pi - \theta_0 + \theta_1) + \theta_2  \\
        \end{array}
        \right..
    \end{equation}

    The solution $\theta_0 = \theta_2 = -\frac{\pi}{4}$ (or $\frac{7\pi}{4}$), $\theta_1=\frac{\pi}{2}$ is feasible. Therefore, we can find a circuit using $K=2$ CNOTs to decompose this rotation table as shown in \Cref{fig:exact-synthesis-mcry}. 

    We can verify $K=1$ has no feasible solution by observing the corresponding equality system in \Cref{eqn:equality-system-no-solution}. 
    \begin{equation}\label{eqn:equality-system-no-solution}
        \left\{
        \begin{array}{rl}
            \varphi^{00}_{1}&=\varphi^{00}_{0} + \theta_1  \\
            \varphi^{01}_{1}&=\varphi^{01}_{0} + \theta_1  \\
            \varphi^{10}_{1}&=\pi - \varphi^{10}_{0} + \theta_1  \\
        \end{array}
        \right. \rightarrow
        \left\{
        \begin{array}{rl}
            0&=\theta_0 + \theta_1  \\
            \frac{\pi}{2}&=\theta_0 + \theta_1 \\
            \frac{3\pi}{2}&=\pi - \theta_0 + \theta_1 \\
        \end{array}
        \right..
    \end{equation}

    Similarly, $K=0$ is also infeasible, and we return the 2-CNOT circuit as the optimal solution. 
\end{example}

\begin{theorem}\label{thm:exact-mcry-decomposition-correctness}
    \Cref{alg:exact-mcry-decomposition} returns the circuit the minimum number of CNOT gates to decompose an MCR$_y$ gate using $\{\text{CNOT}, \text{R}_y\}$ gates. 
\end{theorem}
\begin{proof}
    Since the optimal CNOT number is a natural number, our method would traverse it in one of the iterations between steps 2) and 3). It suffices to show that our equality system in step 2) is equivalent to the existence condition and does not return false positives ($\Rightarrow$) or false negatives ($\Leftarrow$). 

    To prove ($\Rightarrow$), we show that the feasible solution to our system correctly prepares the rotation table in \Cref{eqn:rotation-angle-constraints}. For R$_y$ operators, $\text{R}_y(\theta_1)\text{R}_y(\theta_2) = \text{R}_y(\theta_1+\theta_2)$. Hence, the R$_y$ after each CNOT gate adds a global value to all the entries in the rotation table. For CNOT operators, if the index $\ket{x}$ is enabled, then the state before and after can be expressed as $\ket{x}\otimes(\alpha\ket{0}+\beta\ket{1})$ and $\ket{x}\otimes(\beta\ket{0}+\alpha\ket{1})$. Notice that $\varphi^x_k$ and $\varphi^x_{k+1}-\theta_k$ are the rotation angles before and after $k$th CNOT. Since $\alpha,\beta\in \mathcal{R}$ in our scope, $\varphi^x_{k} + \varphi^x_{k+1} - \theta_k = 2\cdot\arctan\frac{\beta}{\alpha} + 2\cdot\arctan\frac{\beta}{\alpha} = \pi$ holds. Therefore, \Cref{eqn:rotation-angle-constraints} correctly expresses the state transition. 

    To prove ($\Leftarrow$), we must show that our template covers all the possible candidate circuits. Our formulation covers all the combinations of $\{\text{CNOT}, \text{R}_y\}$ because we consider all the control qubits and can merge multiple R$_y$ gates between two adjacent CNOTs. 
\end{proof}

\begin{theorem}\label{thm:exact-mcry-decomposition-complexity}
    The classical time complexity of \Cref{alg:exact-mcry-decomposition} is $\mathcal{O}(n^K\cdot m\cdot K\cdot (n+K))$, where $n$ is the number of control qubits, $m$ is the cardinality of the care set, and $k$ is the optimum CNOT number.
\end{theorem}
\begin{proof}
    The complexity of \Cref{alg:exact-mcry-decomposition} depends on the iteration number of the loop body (lines 5-6) and the complexity of it. 

    Let $k$ be the temporal value of $K$ in the while loop. The for loop at line 4 executes $n^k$ times because we enumerate all the possible sequences of $n$ control qubits with length $k$. 
    
    To construct the equality system, we need to derive the values of all the $R_k^x$ variables using \Cref{eqn:r-s-variable-relation} and plug them into \Cref{eqn:rotation-angle-constraints}. For each $R_k^x, k\in\mathbb{Z}_{K}, x\in\mathbb{Z}_{m}$, the former require $\mathcal{O}(n)$ operations and the later requires $\mathcal{O}(1)$. Therefore, $\mathcal{O}(knm)$ in total. The equality system $M$ at line 5 is a linear system with $K+1$ variables, one for each R$_y$ gate, and $m$ constraints, one for each rotation angle in the care set. Applying the Gaussian elimination algorithm solves the linear system with a time complexity of $\mathcal{O}(k^2m)$.
    
    Therefore, the complexity to solve $K=k$ is $\mathcal{O}(n^k\cdot m\cdot k\cdot (n+k))$ in total. As $k$ increases from $0$ to $K$, the complexity grows faster than the geometric series. Therefore, the asymptotic complexity depends on the largest $k$ we try to solve, $K$.   
\end{proof}

Note that since the Gray code decomposition method guarantees finding a solution with $2^n$ CNOTs, the value of $K$ is upper bounded by $2^n$. However, as observed in the Example~\ref{example:exact-mcry-decomposition}, the linear system has $K+1$ variables and $m$ equality constraints. Therefore, if we can find a template without redundant CNOTs, $K+1=m$ guarantees that the linear system has a solution. By leveraging the don't care in the rotation table, we find a tighter upper bound for the CNOT number to decompose $\text{MCR}_y$, $m-1$. In the worst-case scenario, the cardinality of the care set in the rotation table is $m=2^n$, and our upper bound is reduced to the Gray code decomposition. However, our method reduces the CNOT number significantly for sparse rotation tables.

\todo{Run experiments and demonstrate the results and show the improvement.}

\note{Currently, \Cref{alg:exact-mcry-decomposition} is implemented using Mathematica, as suggested by Daniel. I call the numerical solver ``NMinimize'' to speed up lines 5-6 in the algorithm. As a result, the time complexity is much lower than the formula given in \Cref{thm:exact-mcry-decomposition-complexity}. This points to the potential to develop a numerical method that solves the MCRy decomposition under an error bound.}

\note{Besides, this method can be generalized to multi-target operator synthesis with don't care. In this case, we need to enumerate both the control qubit and target qubit in the templates, and the rotation angle constraints are more complicated. In my current implementation, the Mathematica numerical solver can return the circuit to prepare a 4-qubit state with up to 3 CNOTs in 1 sec, but it is currently not scalable.}
