# Supplementary material for: Quantum State Preparation Using an Exact CNOT Synthesis Formulation
Source: arXiv:2401.01009 source file (2024-01-02)
Supplement: Supplementary file 3 [file appendix-optimality-stap.tex]

\begin{definition}
    We define $\leq$ as a partial order between two libraries $\mathcal{L}_1$ and $\mathcal{L}_2$. $\mathcal{L}_1 \leq \mathcal{L}_2$ if the minimum CNOT number of circuit using $\mathcal{L}_1$ is lower to equal to circuit using $\mathcal{L}_2$ for all real QSP problems. Two libraries are equivalent if $\mathcal{L}_1 \leq \mathcal{L}_2$ and $\mathcal{L}_2 \leq \mathcal{L}_1$ hold.
\end{definition}

By the definition of the CNOT cost, a circuit composed of another library can be decomposed using $\mathcal{L_0} = \{\text{CNOT}, \mathcal{U}(2)\}$ with the same CNOT cost. Therefore, the library $\mathcal{L}_0$ is the smallest element among all the libraries. 

\begin{lemma}\label{lem:cnot-u2-is-mcry}
    $\{\text{CNOT}, \mathcal{U}(2)\} = \{\text{CNOT}, \text{R}_y\} = \{\text{MCR}_y\}$. 
\end{lemma}
\begin{proof}
    The former equality holds because a gate in $\mathcal{U}(2)$ is equivalent to a $\text{R}_y$ according to Observation~\ref{obs:unitary-is-ry}. The latter one holds because we can find the optimal CNOT cost using \Cref{alg:exact-mcry-decomposition}. As proved in Theorem~\ref{thm:exact-mcry-decomposition-correctness}, the CNOT cost of each $\text{MCR}_y$ is the minimum number of CNOT in the decomposition using $\{\text{CNOT}, \text{R}_y\}$. Therefore, for each circuit of $\{\text{CNOT}, \text{R}_y\}$, we can first partition it by the target qubit. Since each partition can be transformed into a $\text{MCR}_y$ gate, the entire circuit can also be implemented using $\{\text{MCR}_y\}$ with the same CNOT cost. 
\end{proof}

Note that the library $\mathcal{L}_{\text{QSP}}$ introduced in \Cref{subsec:library}, $\mathcal{L}_{\text{QSP}}=\{\text{STAP}\}$, is a subset of $\text{MCR}_y$. Hence, $\mathcal{L}_0\!=\!\{\text{MCR}_y\}\!\leq\!\mathcal{L}_{\text{QSP}}$. \note{It is plausible that $\mathcal{L}_0\!=\!\{\text{MCR}_y\}\!=\!\mathcal{L}_{\text{QSP}}$, but I need more time to prove/disprove this.}
