# Supplementary material for: Quantum State Preparation Using an Exact CNOT Synthesis Formulation
Source: arXiv:2401.01009 source file (2024-01-02)
Supplement: Supplementary file 4 [file appendix-optimality.tex]

\section{Optimality of the Exact CNOT Synthesis}
This section discusses the optimality of our exact CNOT synthesis algorithm.
\subsection{Shortest Path Problem Formulation}
With our exact CNOT synthesis formulation, the problem of optimizing CNOT cost for quantum state preparation is equivalent to finding the shortest path between two vertices in the state transition graph. 
\begin{lemma}\label{lemma:two-problems-are-equivalent}
The two problems below are equivalent. 
\begin{itemize}
    \item Prepare $\psi$ using minimum CNOT cost.
    \item Find the shortest path between $\ket{0}$ and $\psi$ in $G_\mathcal{L}$.
\end{itemize}
\end{lemma}

\begin{proof}
By definition, the arcs in $A_G$ correspond one-to-one to quantum operators. Since a path is a sequence of arcs, and a quantum circuit is a sequence of gates, the mapping between paths and quantum circuits is also one-to-one. Besides, the distance of a path is the sum of distances on the arcs, and the CNOT cost of a circuit is the total number of CNOT gates to decompose all the gates. Therefore, the two problems have isomorphic solution spaces and are equivalent. 
\end{proof}

\subsection{A* Algorithm}
Our search algorithm finds the shortest path from the target state to the ground state. The corresponding state transitions are in the opposite direction of the QSP circuit. However, since the quantum operators are reversible, switching the starting and ending point does not affect the shortest path.

\begin{lemma}\label{lemma:cnot-costs-are-equal}
    The CNOT costs of a quantum operator $U$ and its inverse $U^\dagger$ are equal. Therefore, $\gamma(\varphi,\psi)$ and $\gamma(\psi,\varphi)$ have the same minimum value.
\end{lemma}
\begin{proof}
    Let $U=U_1U_2\cdots U_l$ be the decomposition of $U$ using gates in $\{\text{CNOT},\mathcal{U}(2)\}$ that gives the minimum number of CNOTs, $\Delta(U)$. Since $U^\dagger=U_l^\dagger\cdots U_2^\dagger U_1^\dagger$ correctly decompose $U^\dagger$ with the same number of CNOTs, the CNOT cost of $U^\dagger$ is at most $\Delta(U)$, i.e., $\Delta(U^\dagger) \leq \Delta(U)$. Repeat the above procedure on $U^\dagger$ gives $\Delta(U) \leq \Delta(U^\dagger)$. Therefore, $\Delta(U) = \Delta(U^\dagger)$. 
    
    Similarly, if a circuit prepares state $\psi$ from $\varphi$, the inverse of the circuit that prepares $\varphi$ from $\psi$ reverses the order of the quantum gates and conjugates the operators. Therefore, the CNOT cost is the same.
\end{proof}

\subsection{Admissible Heuristic Function}
In \Cref{subsec:a-star}, we introduce a heuristic function to estimate the lower bound of the distance between the current and final states $\ket{0}$. The heuristic counts the number of entangled qubit pairs by evaluating \emph{mutual information} and uses it as the lower bound of the CNOT gate number. If this function is \emph{admissible}, i.e., $\hat\delta(\psi, \ket{0})$ always underestimates the true cost between $\varphi$ and $\ket{0}$, the A* heuristic can prune unpromising branches and improve efficiency without loss in optimality. 

\begin{lemma}\label{lemma:admissible-heuristic}
    If a state $\psi$ has $k$ qubits that have different cofactors, then we need at least $\lceil\frac{k}{2}\rceil$ CNOTs to prepare $\psi$, i.e., $\gamma(\ket{0},\psi) \geq \lceil\frac{k}{2}\rceil$. Therefore, the heuristic $\hat{\delta}(\ket{0},\psi)=\lceil\frac{k}{2}\rceil$ is admissible. 
\end{lemma}
\begin{proof}
    If a qubit $q_i$ is separable in the state $\psi$, then $\psi$ is a product state and can be written as $\ket{\psi} = \ket{\phi}_i\otimes \ket{\varphi}_A = (c_0\ket{0}_i+c_1\ket{1}_i)\otimes \ket{\varphi}_A$, where $A$ represents the remaining system besides $q_i$. The expression implies that the index sets of cofactors $S\left(\left.\psi\right|_{q_i=1}\right) = S\left(\left.\psi\right|_{q_i=0}\right) = S\left(\varphi_A\right)$. Therefore, the contraposition, if the cofactors of $q_i$ are different, then $q_i$ is not separable, holds. 

    Observe that single-qubit gates do not affect the number of entangled qubits, and a CNOT gate can entangle at most two qubits. Therefore, when preparing a state $\psi$ with $k$ entangled qubits, we need at least $\lceil\frac{k}{2}\rceil$ CNOT gates.
\end{proof}

\subsection{Optimality of the Exact CNOT Synthesis}
\begin{theorem}
    \Cref{alg:bfs} returns the optimal circuit composed by gates in the given library $\mathcal{L}$ with minimum CNOT cost.
    % provided that the CNOT costs of gates indicate the optimal CNOT number to decompose it. (not necessary)
\end{theorem}
\begin{proof}
According to Lemma~\ref{lemma:two-problems-are-equivalent} and Lemma~\ref{lemma:cnot-costs-are-equal}, the shortest path between $\psi$ and $\ket{0}$ represents the optimal circuit with the minimum CNOT cost. We have demonstrated in Lemma~\ref{lemma:admissible-heuristic} that our heuristic estimation is admissible. To complete the proof, it suffices to show the state compression method does not affect the optimality.

Let $\psi_0$ be the target state, and $\varphi$ be a state pruned by state compression. By definition, the representative of $\varphi$, $\Pi(\varphi)$, is enqueued with a distance $\gamma(\psi_0, \Pi(\varphi)) \leq \gamma(\psi_0, \varphi)$. Since $\varphi$ and $\Pi(\varphi)$ are equivalent and can be prepared using the same number of CNOT gates, $\gamma(\ket{0}, \Pi(\varphi)) = \gamma(\ket{0}, \varphi)$. Notice that if $\varphi$ is not on the shortest path, pruning it does not affect the optimal distance. Then, assume $\varphi$ is on the shortest path between $\psi_0$ and $\ket{0}$, then $\gamma(\ket{0}, \psi_0) = \gamma(\ket{0}, \varphi) + \gamma(\varphi, \psi_0)$ holds. However, $\gamma(\ket{0}, \Pi(\varphi)) + \gamma(\varphi, \Pi(\psi_0)) \leq \gamma(\ket{0}, \psi_0)$, which implies a path with same optimal distance can be found through $\Pi(\varphi)$ if $\varphi$ is pruned. Therefore, we conclude that the state compression would not affect the optimal value.
\end{proof}
